# Supplementary material for: Cost-based Selection of Provenance Sketches for Data Skipping
Source: arXiv:2504.19252 source file (2025-04-27)
Supplement: Supplementary file 1 [file appendix.tex]

\section{Appendix}
 \begin{figure}
    \centering 
    \includegraphics[width=3in]{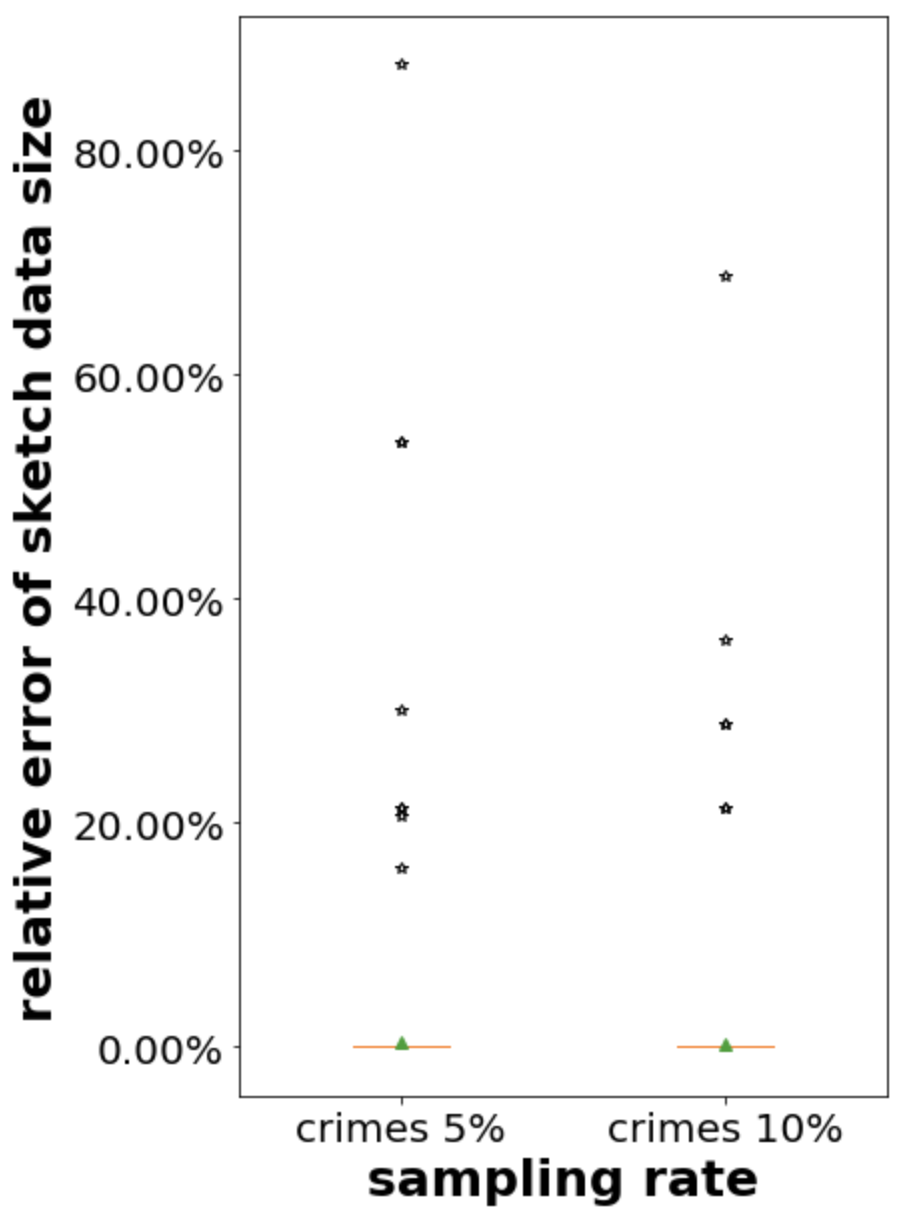}
    \caption{relative error of sketch data size varying sampling rate over CRIMES} 
    \label{relative_error_crimes}
\end{figure}

\begin{figure}
    \centering 
    \includegraphics[width=3in]{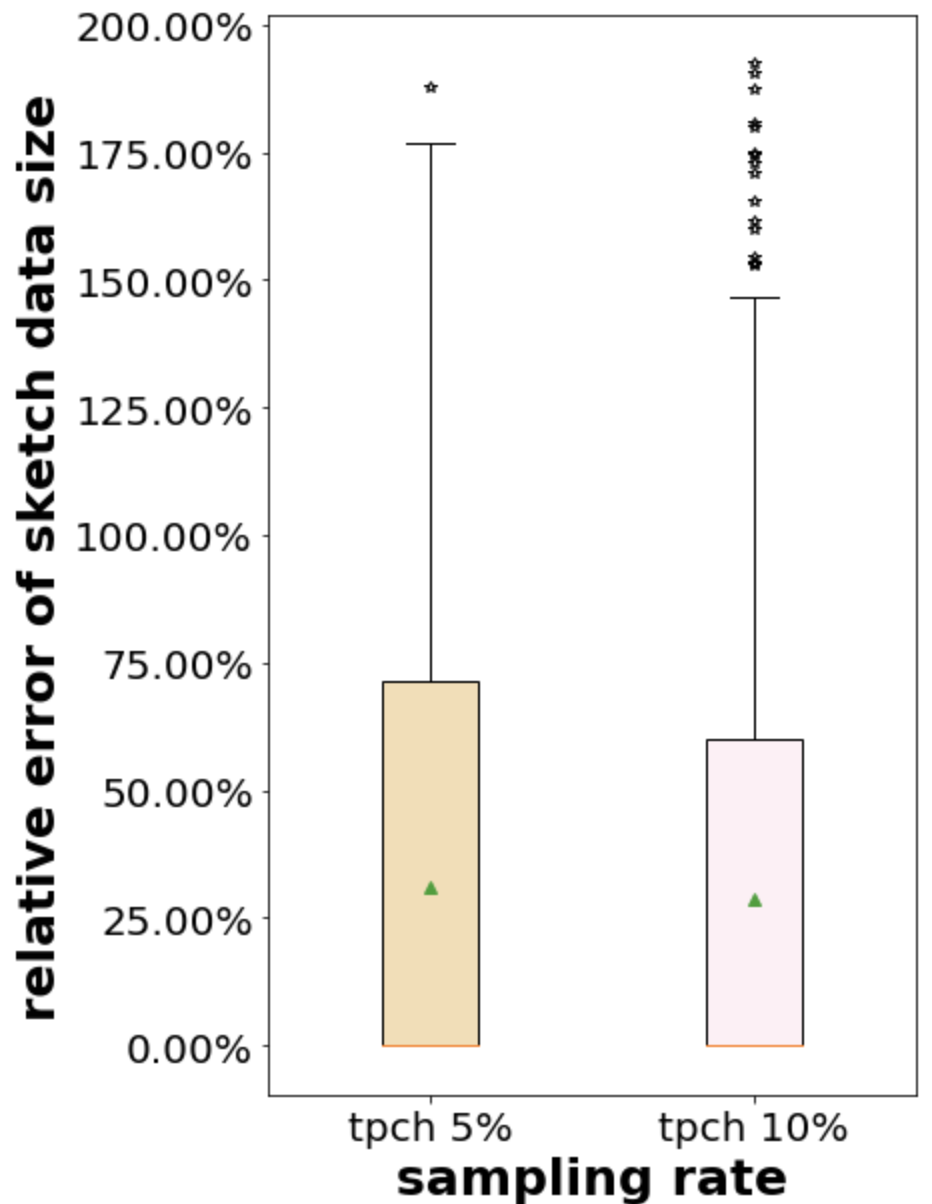}
    \caption{relative error of sketch data size varying sampling rate over TPCH} 
    \label{relative_error_tpch}
\end{figure}

\begin{figure}
    \centering 
    \includegraphics[width=3in]{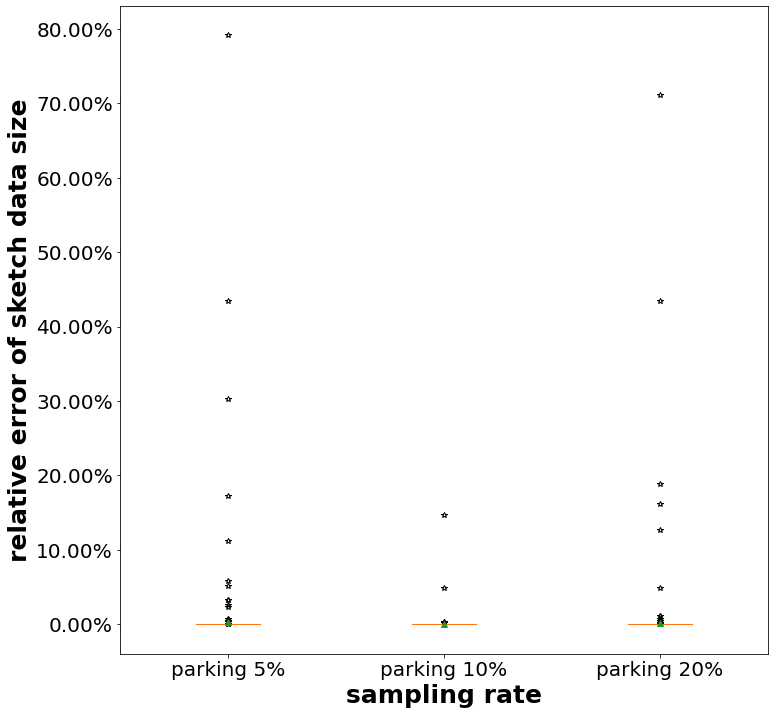}
    \caption{relative error of sketch data size varying sampling rate over PARKING} 
    \label{relative_error_parking}
\end{figure}

\begin{figure}
    \centering 
    \includegraphics[width=3in]{pic/running_time_comparation_crimes.png}
    \caption{Average running time of query vs different strategies over CRIMES} 
    \label{running_time_comparation_crimes}
\end{figure}

\begin{figure}
    \centering 
    \includegraphics[width=3in]{pic/running_time_comparation_tpch.png}
    \caption{Average running time of query vs different strategies over TPCH} 
    \label{running_time_comparation_tpch}
\end{figure}

\begin{figure}
    \centering 
    \includegraphics[width=3in]{pic/running_time_comparation.png}
    \caption{Average running time of query vs different strategies over PARKING} 
    \label{running_time_comparation_parking}
\end{figure}

\begin{figure}
    \centering 
    \includegraphics[width=3in]{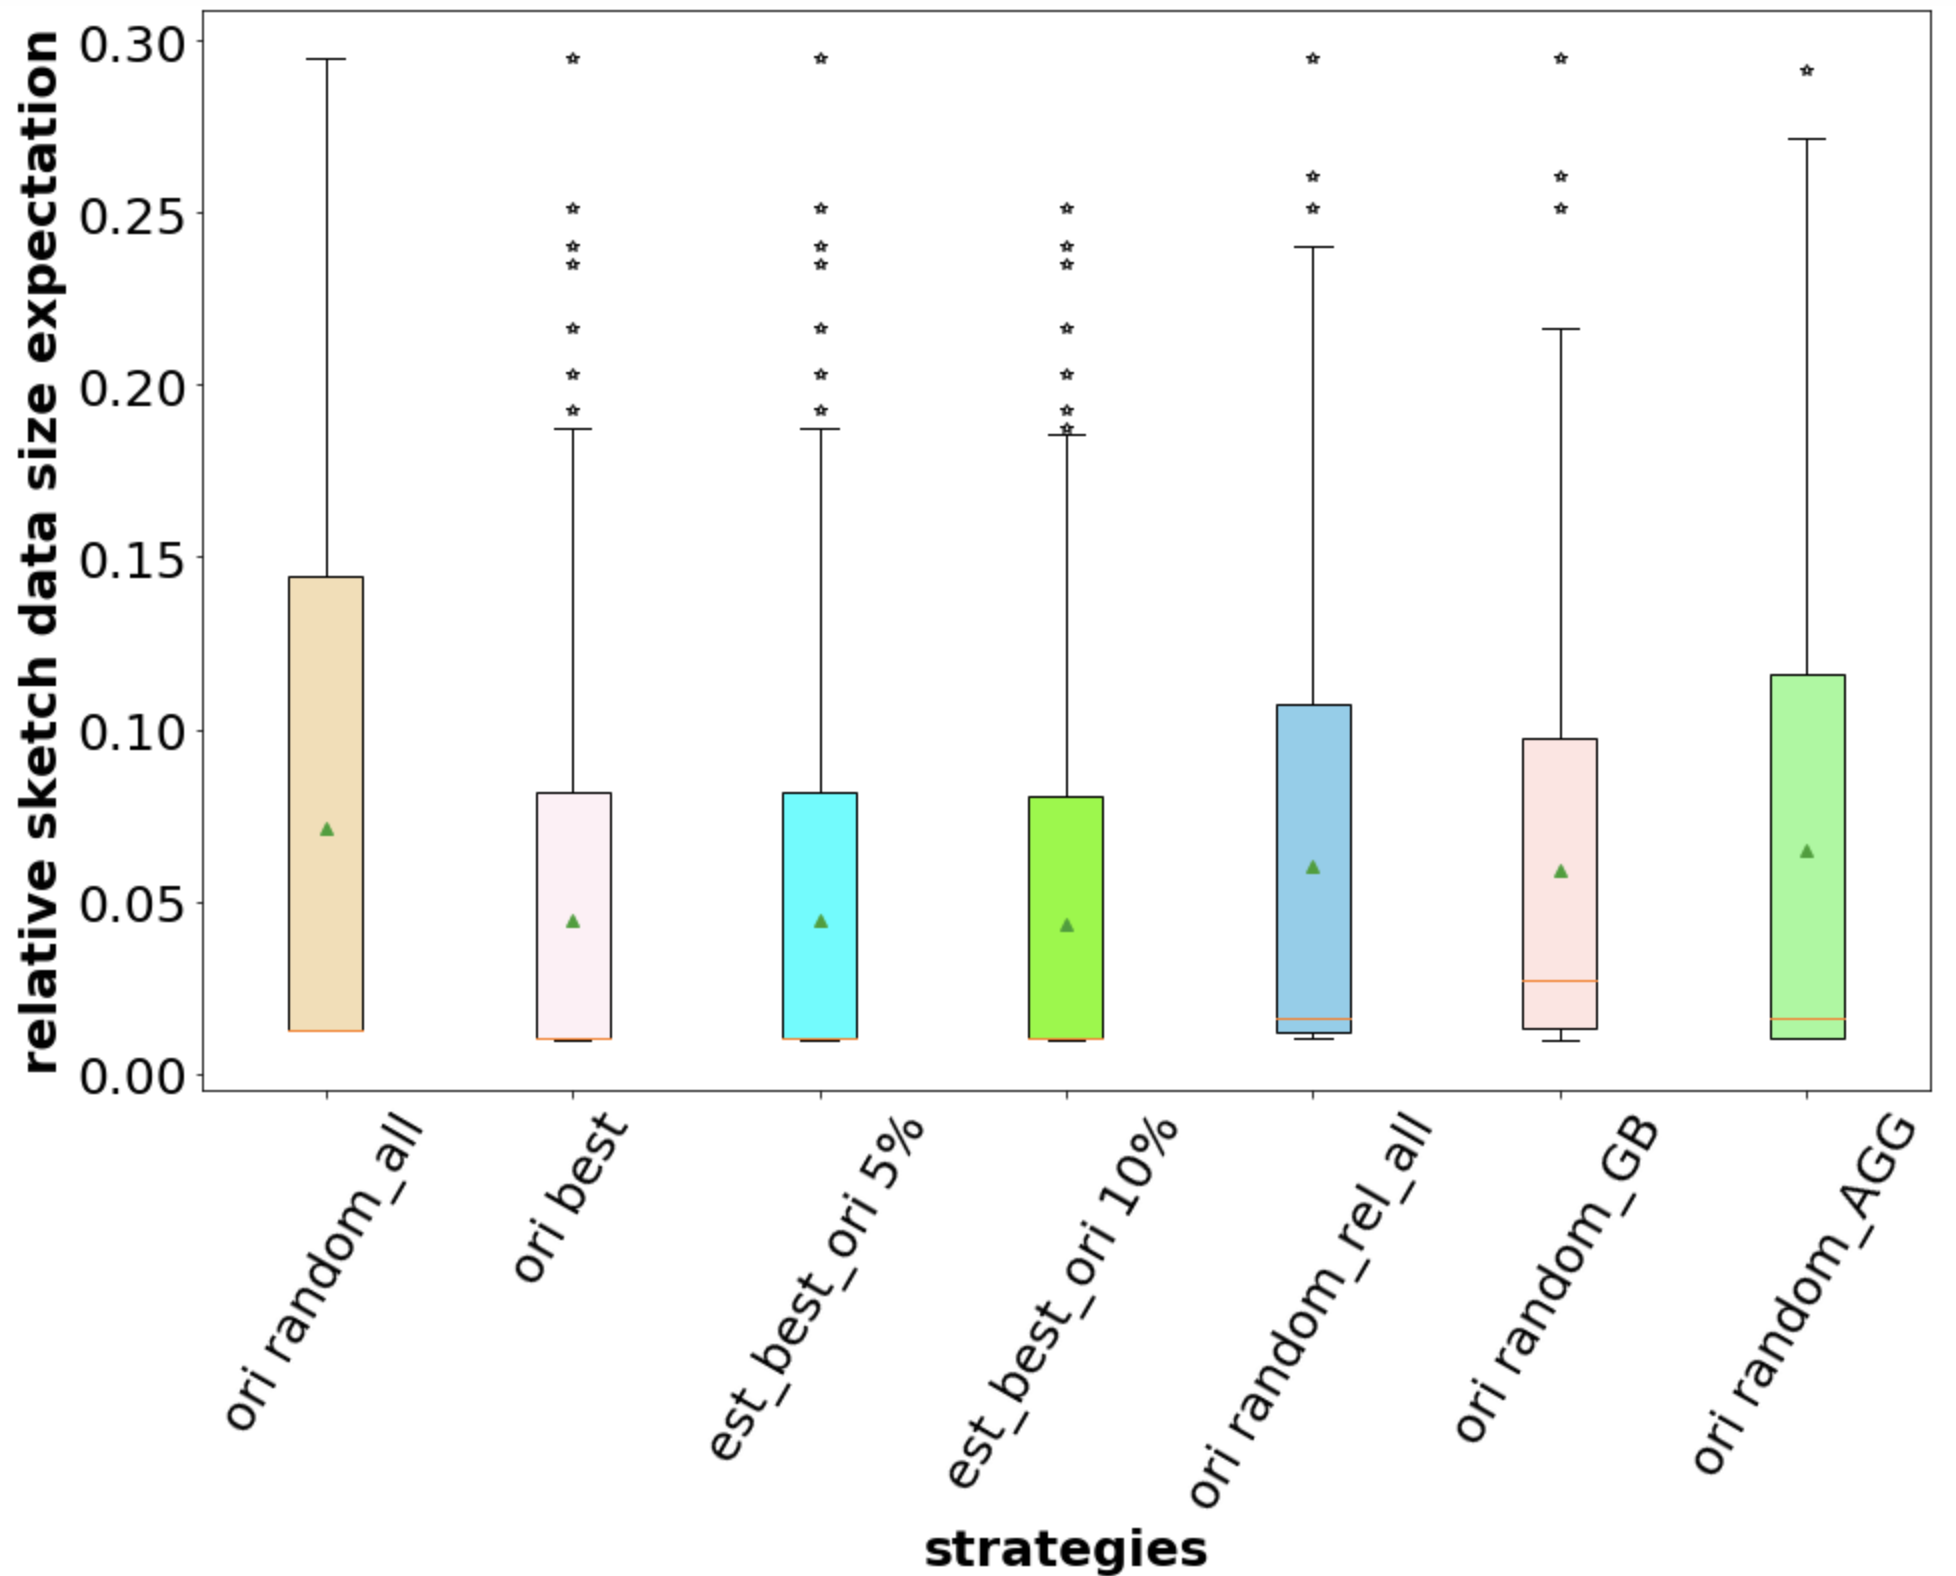} 
    \caption{Relative sketch data size expectation varying strategies over CRIMES} 
    \label{box_plot_crimes} 
\end{figure}

\begin{figure}
    \centering 
    \includegraphics[width=3in]{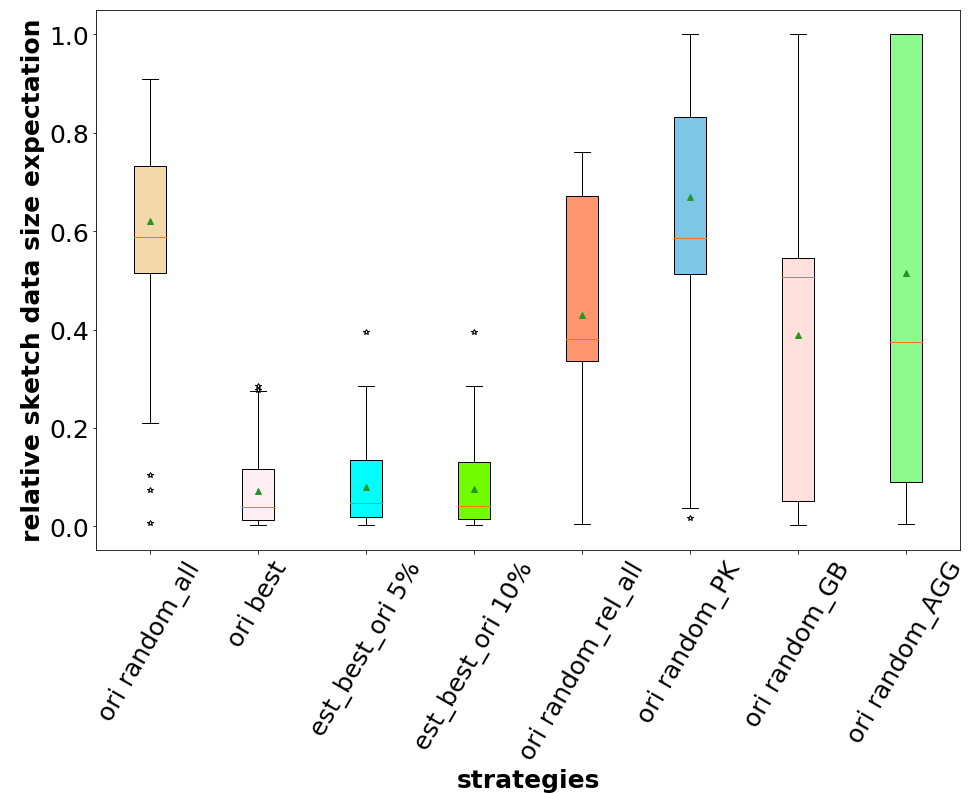} 
    \caption{Relative sketch data size expectation varying strategies over TPCH} 
    \label{box_plot_tpch} 
\end{figure}

\begin{figure}
    \centering 
    \includegraphics[width=3in]{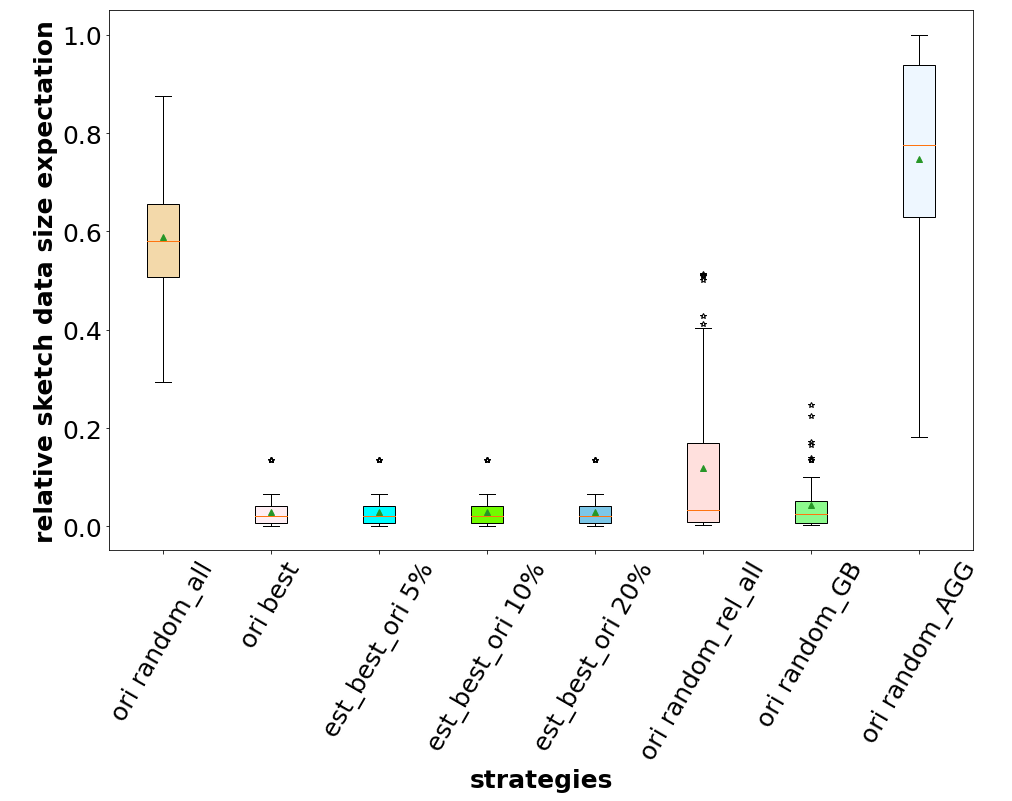} 
    \caption{Relative sketch data size expectation varying strategies over PARKING} 
    \label{box_plot_parking} 
\end{figure}

\begin{figure}
    \centering 
    \includegraphics[width=3in]{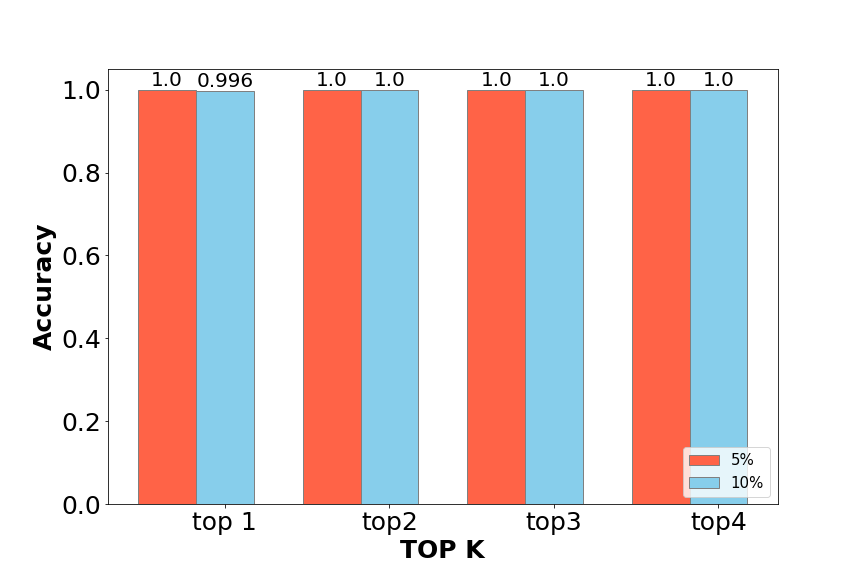}
    \caption{Accuracy of estimation of top k attribute over the CRIMES varying k} 
    \label{accuracy_crimes_bar} 
\end{figure}

\begin{figure}
    \centering 
    \includegraphics[width=3in]{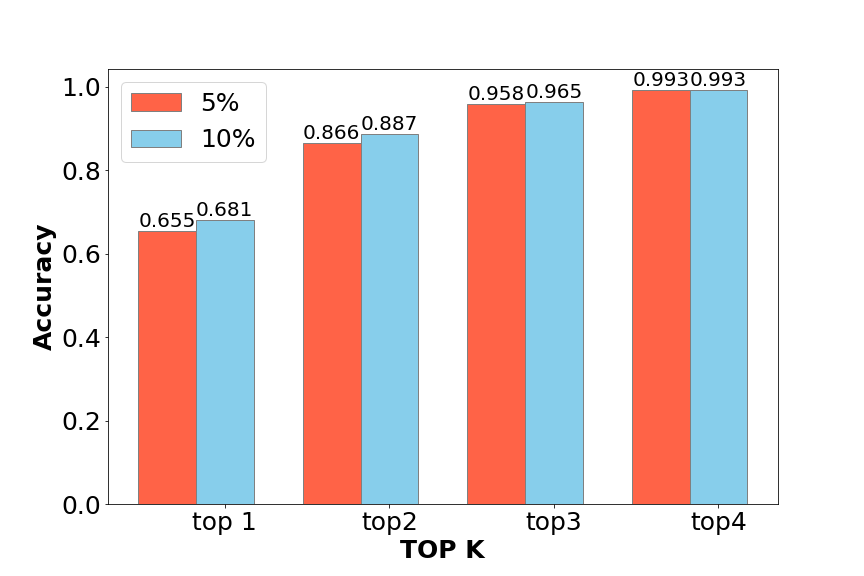} 
    \caption{Accuracy of estimation of top k attribute over the TPCH varying k} 
    \label{accuracy_tpch_bar} 
\end{figure}

\begin{figure}
    \centering 
    \includegraphics[width=3in]{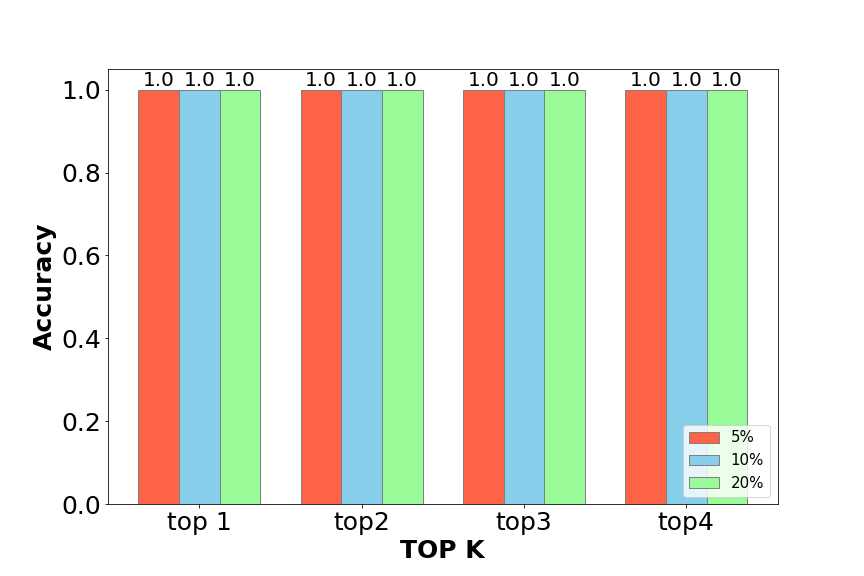} 
    \caption{Accuracy of estimation of top k attribute over the PARKING varying k} 
    \label{accuracy_parking_bar} 
\end{figure}

\begin{figure}
    \centering 
    \includegraphics[width=3in]{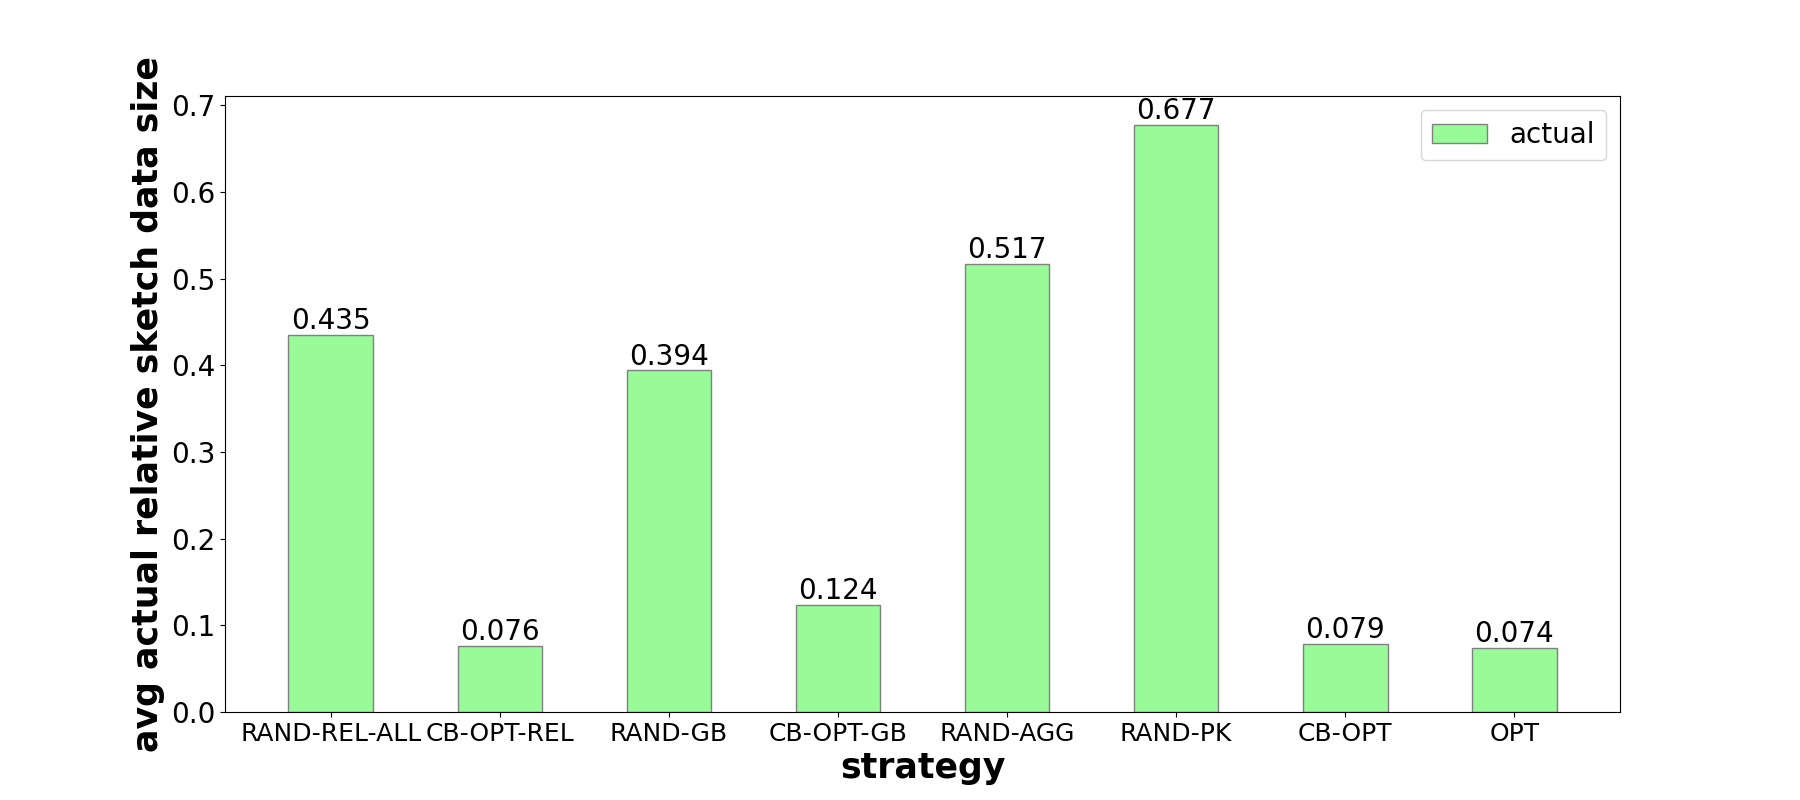}
    \caption{Average relative sketch data size over TPCH} 
    \label{AVG_sketch_selectity_TPCH}
\end{figure}

\begin{figure}
    \centering 
    \includegraphics[width=3in]{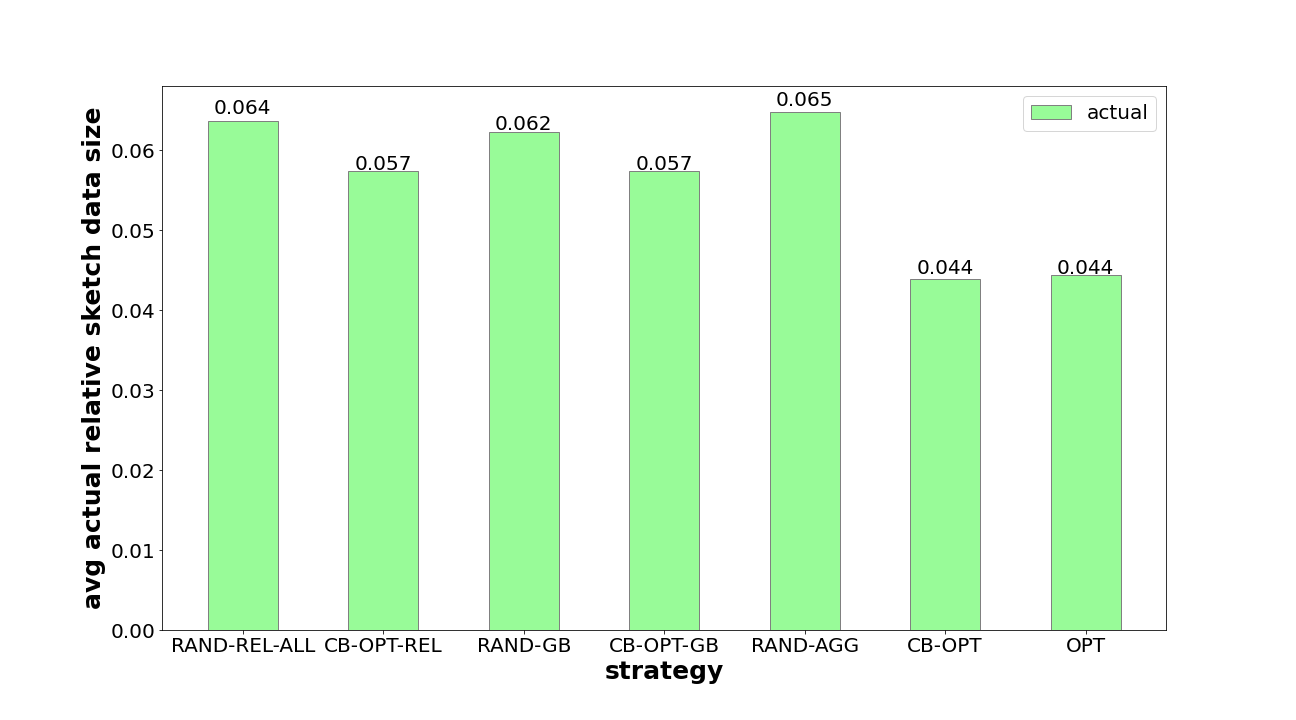}
    \caption{Average relative sketch data size over CRIMES} 
    \label{AVG_sketch_selectity_crimes}
\end{figure}

\begin{figure}
    \centering 
    \includegraphics[width=3in]{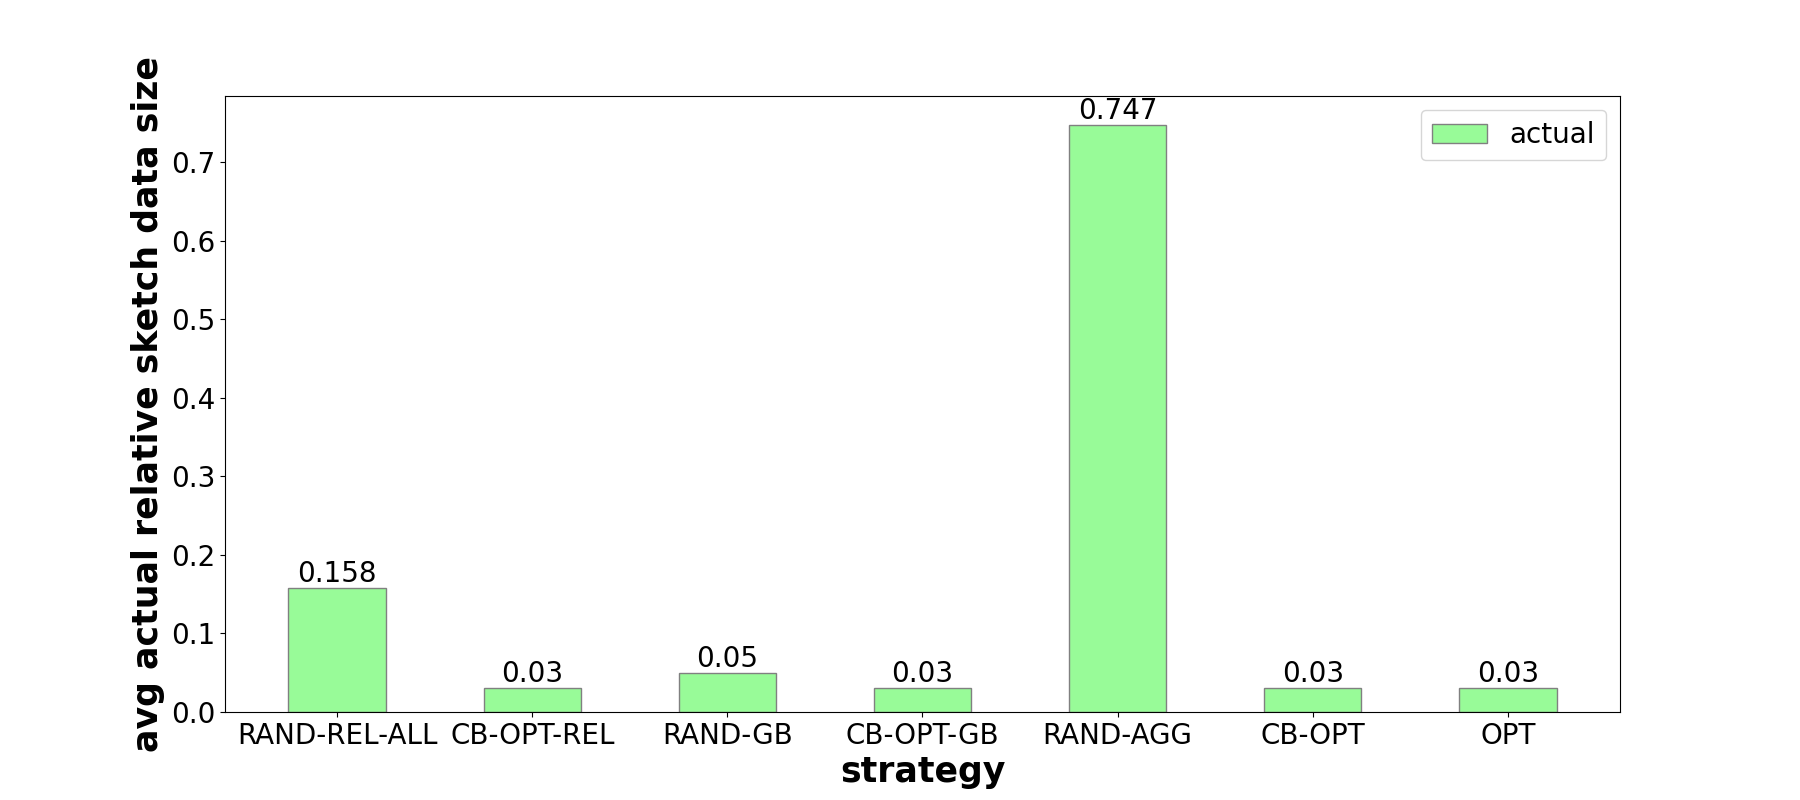}
    \caption{Average relative sketch data size over PARKING} 
    \label{AVG_sketch_selectity_parking}
\end{figure}

%%%%%%%%%%%%%%%%%%%%%%%%%%%%%%%%%%%%%%%%%%%%%%%%%%%%%%%%%%%%%%%%%%%%%%%%%%%%%%%%

\begin{figure}
    \centering 
    \includegraphics[width=3in]{pic/end-to-end-3gb-all-strategies-2percent.png}
    \caption{cumulative time of all strategies of selection-aggregation queries with 3 group by over TPCH 2\%} 
    \label{end-to-end-different-strategies-3gb-2percent}
\end{figure}

\begin{figure}
    \centering 
    \includegraphics[width=3in]{pic/end-to-end-all-strategies-wdj-3gb.png}
    \caption{cumulative time of all strategies of selection-aggregation-join queries with 3 group by over TPCH} 
    \label{end-to-end-different-strategies-wdj-3gb}
\end{figure}

\begin{figure}
    \centering 
    \includegraphics[width=3in]{pic/end-to-end-all-strategies-complex.png}
    \caption{cumulative time of all strategies of complex queries with 2 group by over TPCH} 
    \label{end-to-end-different-strategie-complex}
\end{figure}

\begin{figure}
    \centering 
    \includegraphics[width=3in]{pic/end-to-end-all-strategies-complex-3gb.png}
    \caption{cumulative time of all strategies of complex queries with 3 group by over TPCH} 
    \label{end-to-end-different-strategies-complex-3gb}
\end{figure}

\begin{figure}
    \centering 
    \includegraphics[width=3in]{pic/end-to-end-all-strategies-stars-2gb.png}
    \caption{cumulative time of all strategies of selection-aggregation queries with 2 group by over stars} 
    \label{end-to-end-different-strategies-complex-3gb}
\end{figure}

\begin{figure}
    \centering 
    \includegraphics[width=3in]{pic/stars.png}
    \caption{Average relative sketch data size over Stars } 
    \label{Average-relative-sketch-data-size-over-stars }
\end{figure}

\begin{figure}
    \centering 
    \includegraphics[width=3in]{pic/running_overhead.png}
    \caption{running time for each step} 
    \label{running_overhead}
\end{figure}

\begin{figure}
    \centering 
    \includegraphics[width=3in]{pic/parking.png}
    \caption{clustering of parking} 
    \label{clustering_parking}
\end{figure}

\begin{figure}
    \centering 
    \includegraphics[width=3in]{pic/Average_relative_sketch_data_size_clustering_parking.png}
    \caption{Relative average sketch data size clustering of parking} 
    \label{Average_relative_sketch_data_size_clustering_parking}
\end{figure}

\begin{figure}
    \centering 
    \includegraphics[width=3in]{pic/Average_relative_sketch_data_size__clustering_crimes.png}
    \caption{Relative average sketch data size clustering of CRIMES} 
    \label{Average_relative_sketch_data_size__clustering_crimes}
\end{figure}

\begin{figure}
    \centering 
    \includegraphics[width=3in]{pic/difference_of_each_candidate_crimes.png}
    \caption{difference of each candidate of CRIMES} 
    \label{difference_of_each_candidate_crimes}
\end{figure}

\begin{figure}
    \centering 
    \includegraphics[width=3in]{pic/difference_of_each_candidate_parking.png}
    \caption{difference of each candidate of PARKING} 
    \label{difference_of_each_candidate_parking}
\end{figure}

%%%%%%%%%%%%%%%%%%%%%%%%%%%%%%%%%%%%%%%%%%%%%%%%%%%%%%%%%%%%%%%%%%%%%%%%%%%%%%%%
%\begin{figure}
%    \centering 
%    \includegraphics[width=3in]{pic/running_time_comparation_crimes.png}
%    \caption{Average running time of query vs different strategies over CRIMES} 
%    \label{running_time_comparation_crimes}
%\end{figure}
%
%\begin{figure}
%    \centering 
%    \includegraphics[width=3in]{pic/running_time_comparation_tpch.png}
%    \caption{Average running time of query vs different strategies over TPCH} 
%    \label{running_time_comparation_tpch}
%\end{figure}
%
%\begin{figure}
%    \centering 
%    \includegraphics[width=3in]{pic/running_time_comparation.png}
%    \caption{Average running time of query vs different strategies over PARKING} 
%    \label{running_time_comparation_parking}
%\end{figure}

%%%%%%%%%%%%%%%%%%%%%%%%%%%%%%%%%%%%%%%%%%%%%%%%%%%%%%%%%%%%%%%%%%%%%%%%%%%%%%%%

\begin{figure}
    \centering 
    \includegraphics[width=3in]{pic/Best_choice_distribution_crimes.png}
    \caption{Best choice distribution over CRIMES} 
    \label{Best_choice_distribution_crimes}
\end{figure}

\begin{figure}
    \centering 
    \includegraphics[width=3in]{pic/Best_choice_distribution_tpch.png}
    \caption{Best choice distribution over TPCH} 
    \label{Best_choice_distribution_tpch}
\end{figure}

\begin{figure}
    \centering 
    \includegraphics[width=3in]{pic/Best_choice_distribution_parking.png}
    \caption{Best choice distribution over PARKING} 
    \label{Best_choice_distribution_parking}
\end{figure}

%%%%%%%%%%%%%%%%%%%%%%%%%%%%%%%%%%%%%%%%%%%%%%%%%%%%%%%%%%%%%%%%%%%%%%%%%%%%%%%%

\clearpage

\begin{figure}
    \centering 
    \includegraphics[width=3in]{pic/box_plot_tpch_wanderjoin.png} 
    \caption{Relative sketch data size expectation varying strategies over TPCH WANDER JOIN} 
    \label{box_plot_tpch_wanderjoin} 
\end{figure}

\begin{figure}
    \centering 
    \includegraphics[width=3in]{pic/accuracy_tpch_bar_wanderjoin.png}
   	\caption{Accuracy of estimation of top k attribute over the TPCH varying k wander join} 
    \label{accuracy_tpch_bar_wanderjoin} 
 \end{figure}

\begin{figure}
    \centering 
    \includegraphics[width=3in]{pic/Average_relative_sketch_data_size_TPCH_wanderjoin.png}
    \caption{Average relative sketch data size over TPCH wander join} 
    \label{AVG_sketch_selectity_TPCH_wanderjoin}
\end{figure}

\begin{figure}
    \centering 
    \includegraphics[width=3in]{pic/relative_error_tpch_wanderjoin.png}
    \caption{relative error of sketch data size varying sampling rate over TPCH wander join} 
    \label{relative_error_tpch_wanderjoin}
\end{figure}

\begin{figure}
    \centering 
    \includegraphics[width=3in]{pic/Best_choice_distribution_tpch_wanderjoin.png}
    \caption{Best choice distribution over TPCH wander join} 
    \label{Best_choice_distribution_tpch_wanderjoin}
\end{figure}

%%%%%%%%%%%%%%%%%%%%%%%%%%%%%%%%%%%%%%%%%%%%%%%%%%%%%%%%%%%%%%%%%%%%%%%%%%%%%%%%
\begin{figure}
    \centering 
    \includegraphics[width=3in]{pic/box_plot_tpch_wanderjoin_3.png} 
    \caption{Relative sketch data size expectation varying strategies over TPCH WANDER JOIN 3} 
    \label{box_plot_tpch_wanderjoin3} 
\end{figure}

\begin{figure}
    \centering 
    \includegraphics[width=3in]{pic/accuracy_tpch_bar_wanderjoin_3.png}
   	\caption{Accuracy of estimation of top k attribute over the TPCH varying k wander join 3} 
    \label{accuracy_tpch_bar_wanderjoin3} 
 \end{figure}

\begin{figure}
    \centering 
    \includegraphics[width=3in]{pic/Average_relative_sketch_data_size_TPCH_wanderjoin_3.png}
    \caption{Average relative sketch data size over TPCH wander join 3} 
    \label{AVG_sketch_selectity_TPCH_wanderjoin3}
\end{figure}

\begin{figure}
    \centering 
    \includegraphics[width=3in]{pic/relative_error_tpch_wanderjoin_3.png}
    \caption{relative error of sketch data size varying sampling rate over TPCH wander join 3} 
    \label{relative_error_tpch_wanderjoin3}
\end{figure}

\begin{figure}
    \centering 
    \includegraphics[width=3in]{pic/Best_choice_distribution_tpch_wanderjoin_3.png}
    \caption{Best choice distribution over TPCH wander join 3} 
    \label{Best_choice_distribution_tpch_wanderjoin3}
\end{figure}
%%%%%%%%%%%%%%%%%%%%%%%%%%%%%%%%%%%%%%%%%%%%%%%%%%%%%%%%%%%%%%%%%%%%%%%%%%%%%%%%
\begin{figure}
    \centering 
    \includegraphics[width=3in]{pic/Running time of reuse over CRIMES.png}
    \caption{Running time of reuse over CRIMES} 
    \label{Running_time_of_reuse_over_CRIMES}
\end{figure}

\begin{figure}
    \centering 
    \includegraphics[width=3in]{pic/Running time of reuse over TPCH.png}
    \caption{Running time of reuse over TPCH} 
    \label{Running_time_of_reuse_over_TPCH}
\end{figure}
%%%%%%%%%%%%%%%%%%%%%%%%%%%%%%%%%%%%%%%%%%%%%%%%%%%%%%%%%%%%%%%%%%%%%%%%%%%%%%%%
\begin{figure}
    \centering 
    \includegraphics[width=3in]{pic/topk_difference_tpch.png}
    \caption{Relative difference of top K PS attributes over tpch} 
    \label{topk_difference_tpch}
\end{figure}

\begin{figure}
    \centering 
    \includegraphics[width=3in]{pic/topk_difference_crimes.png}
    \caption{Relative difference of top K PS attributes over crimes} 
    \label{topk_difference_crimes}
\end{figure}

\begin{figure}
    \centering 
    \includegraphics[width=3in]{pic/topk_difference_parking.png}
    \caption{Relative difference of top K PS attributes over PARKING} 
    \label{topk_difference_parking}
\end{figure}

%%%%%%%%%%%%%%%%%%%%%%%%%%%%%%%%%%%%%%%%%%%%%%%%%%%%%%%%%%%%%%%%%%%%%%%%%%%%%%%%
\begin{figure}
    \centering 
    \includegraphics[width=3in]{pic/end-to-end.png}
    \caption{cumulative time for end-to-end experiments over TPCH} 
    \label{end-to-end}
\end{figure}

\begin{figure}
    \centering 
    \includegraphics[width=3in]{pic/end-to-end-gb.png}
    \caption{cumulative time for end-to-end experiments for group by attributes over TPCH} 
    \label{end-to-end-gb}
\end{figure}

\begin{figure}
    \centering 
    \includegraphics[width=3in]{pic/end-to-end-pk.png}
    \caption{cumulative time for end-to-end experiments for primary key attributes over TPCH} 
    \label{end-to-end-pk}
\end{figure}

\begin{figure}
    \centering 
    \includegraphics[width=3in]{pic/end-to-end-5times.png}
    \caption{cumulative time for end-to-end experiments over TPCH filtered} 
    \label{end-to-end-5t}
\end{figure}

\begin{figure}
    \centering 
    \includegraphics[width=3in]{pic/end-to-end-gb-5times.png}
    \caption{cumulative time for end-to-end experiments for group by attributes over TPCH filtered} 
    \label{end-to-end-gb-5t}
\end{figure}

\begin{figure}
    \centering 
    \includegraphics[width=3in]{pic/end-to-end-pk-5times.png}
    \caption{cumulative time for end-to-end experiments for primary key attributes  over TPCH filtered} 
    \label{end-to-end-pk-5t}
\end{figure}

%\begin{figure}
%    \centering 
%    \includegraphics[width=3in]{pic/end-to-end-different-strategies.png}
%    \caption{cumulative time for end-to-end experiments for different strategies over TPCH filtered} 
%    \label{end-to-end-different-strategies}
%\end{figure}
%%%%%%%%%%%%%%%%%%%%%%%%%%%%%%%%%%%%%%%%%%%%%%%%%%%%%%%%%%%%%%%%%%%%%%%%%%%%%%%%
\begin{figure}
    \centering 
    \includegraphics[width=3in]{pic/number_of_ps.png}
    \caption{cumulative number of PS over TPCH} 
    \label{number_of_pst}
\end{figure}

\begin{figure}
    \centering 
    \includegraphics[width=3in]{pic/times_of_reused.png}
    \caption{times of reused for each PS over TPCH} 
    \label{times_of_reused}
\end{figure}

%%%%%%%%%%%%%%%%%%%%%%%%%%%%%%%%%%%%%%%%%%%%%%%%%%%%%%%%%%%%%%%%%%%%%%%%%%%%%%%%
%%%%%%%%%%%%%%%%%%%%%%%%%%%%%%%%%%%%%%%%%%%%%%%%%%%%%%%%%%%%%%%%%%%%%%%%%%%%%%%%
\clearpage
\section{Experiments}
\label{sec:experiments}
The main goals of this experimental evaluation is to learn the impact of parameters such as number of fragments on the precision and overhead of provenance sketches, and evaluate the accuracy of cost model choosing provenance sketches. All experiments were run on a machine with 2 x 3.3Ghz AMD Opteron 4238 CPUs (12 cores in total) and 128GB RAM running Ubuntu 18.04 (linux kernel 4.15.0). We use Postgres 11.4 as an example of a classical disk-based system.
\subsection{Workloads}
\label{sec:dataset}

\parttitle{Chicago Crime} This dataset records crimes reported in Chicago (\url{https://data.cityofchicago.org/Public-Safety/Crimes-2001-to-present/ijzp-q8t2}). It contains $\sim$6.7M tuples each corresponding to a single crime. %For each crime, the dataset records a unique identifier, the type of the crime, the date, and various geographical attributes (e.g., police district).

\parttitle{TPC-H} The TPC-H is a decision support benchmark. It consists of a suite of business oriented ad-hoc queries and concurrent data modifications.

\parttitle{Parking} This dataset records parking reports in New York City. It contains $\sim$31M tuples.

\parttitle{Stars} We obtained this dataset from SDSS-V. SDSS-V is the first facility providing multi-epoch optical \& IR spectroscopy across the entire sky, as well as offering contiguous integral-field spectroscopic coverage of the Milky Way and Local Volume galaxies. It contains $\sim$5.2M tuples.

\parttitle{Auto-generated queries} We generate 1000 queries for which is based on the selection-aggregation-groupby, selection-aggregation-join-groupby template over the CRIMES, TPCH and PARKING. The query below is a example of the template over CRIMES. We run these queries on our cost model to test the effectiveness and accuracy.\\
\begin{minipage}{0.99\linewidth}
\captionsetup{singlelinecheck = false, justification=justified}
\lstset{upquote=true,frame=single, title = \bf{Q-EXAMPLE, selection-groupby template }}
\begin{lstlisting}
SELECT A,B,AGG(C) AS AGG_C 
FROM CRIMES
GROUP BY A.B
HAVING AGG_C > CONTANT
\end{lstlisting}
\end{minipage}\\
\begin{minipage}{0.99\linewidth}
\captionsetup{singlelinecheck = false, justification=justified}
\lstset{upquote=true,frame=single, title = \bf{Q-EXAMPLE, selection-aggregation-join-groupby template }}
\begin{lstlisting}
SELECT A,B,AGG(C) AS AGG_C 
FROM LINEITEM JOIN ORDERS ON L_ORDERKEY = O_ORDERKEY
GROUP BY A.B
HAVING AGG_C > CONTANT
\end{lstlisting}
\end{minipage}

%\subsection{Test cases}
%1.varying the number of PS for same query to measure the overhead of capture and use \\
%2.experiment of simple queries on CRIMES and MOIVES varying the number fragments to measure the accuracy of cost model only using histogram or only using stratified sampling\\
%3.experiment of complicated queries on CRIMES and MOIVES varying the number fragments to measure the accuracy of cost model  only using histogram or only using stratified sampling\\
%4.experiment of complicated queries on CRIMES and MOIVES varying the number fragments to measure the accuracy of cost model combing histogram and stratified sampling\\
%5.comparing the overhead of candidates,(random choosing, choosing attribute with the most distinct value, choosing the attribute in the group by or selection condition)
\subsection{Strategies}
\label{Strategies}
After the safe provenance sketch attribute candidates are selected by the safety rules. Based on our experiment experience, for the most cases, the performance of the attribute which has small distinct value number is much worse than the performance of the attribute which has large distinct value number. Thus, for our experiments, we firstly have a pre-filtering of the candidates of attribute, filtering the attribute which has fewer distinct value. Many strategies can be applied to choose the optimal attribute for provenance sketch.  Different strategies include random picking from all attributes candidates after pre-filtering which is notated as \textbf{RAN-ALL}, random picking from query-relatively attributes which is notated as \textbf{RAN-REL-ALL}, random picking from group-by attributes which is notated as \textbf{RAN-GB}, random picking from primary key attributes which is notated as \textbf{RAN-PK}. random picking from aggregation attributes which is notated as \textbf{RAN-AGG}. The random picking strategy is that we choose the attributes for provenance sketches from the candidates using the uniform assumption. For example, for random picking from primary key, we uniformly random choose one attribute from all the primary key attributes for provenance sketch. The \textbf{CB-OPT-REL} strategy involves selecting the relative attributes based on the cost-based optimal approach. The \textbf{CB-OPT-GB} strategy involves selecting the group by attribute based on the cost-based optimal approach. The \textbf{CB-OPT} strategy involves selecting the best one based on the cost-based optimal approach.

\subsection{Measuring}
In this section, we will talk about what our experiments measure. We run the auto-generated queries over CRIMES and TPCH and applied our cost model to calculate the sketch data size. First, we measures the relative error for our estimated sketch data size and actual sketch data size to evaluate the effectiveness of our approach. We plot Fig.\ref{relative_error_crimes} and \ref{relative_error_tpch}, relative error for auto-generated queries over CRIMES and TPCH. \\
	Second, we measures the accuracy of of estimation of top k attribute over the CRIMES and TPCH. Our cost model will return the provenance sketch attribute in ascending order based on the relative sketch data size. The relative sketch data size is the fraction of the data size, which measures the rate of how many tuple in dataset are included in the provenance sketch. The meaning of accuracy is that the rate of how many queries return the same optimal attribute using cost model as actual optimal attribute. In addition to the previously described experimental setup, determining the appropriate value of k is a trade-off process. Estimating the optimal attribute is not always accurate, which means we may miss the best sketch candidate by only considering the top-1 attribute. In order to overcome this limitation, we extend our experiments to include the top-k attributes, even though this may result in a higher running overhead. By varying the value of k, we aim to strike a balance between performance and overhead, allowing for a higher chance of finding the best sketch while still maintaining reasonable running costs. To investigate this trade-off, we conduct experiments with different values of k and record the corresponding performance and overhead and plots in Fig.\ref{accuracy_crimes_bar} and \ref{accuracy_tpch_bar}. This way, we can better understand the relationship between k, accuracy, and overhead, and determine an optimal trade-off for our cost model.\\
	Next, we evaluate the actual average relative sketch data size for each strategy discussed in Section \ref{Strategies}. By analyzing the average relative sketch data size, we can compare the effectiveness and benefits of the different strategies more thoroughly. These results are visualized in Fig.\ref{AVG_sketch_selectity_TPCH} and \ref{AVG_sketch_selectity_crimes}.\\
Furthermore, we assess the relative sketch data size expectation for each strategy. To do this, we compute the relative sketch data size for each attribute across all strategies and queries. The expectation is calculated as $E = \sum^n_i r(i)*p(i)$, where $i$ represents the attribute candidate, $r(i)$ denotes the relative sketch data size of one candidate, and $p(i)$ is the weight for each attribute candidate. For random picking, we make the assumption of uniform distribution. The expectations for each strategy are illustrated in Fig.\ref{box_plot_crimes} and \ref{box_plot_tpch}.\\
Apart from the relative sketch data size, we also examined the average running time of queries for different strategies. In this test, we captured, used and ran queries with provenance sketches based on the selection of various strategies. We observed that the results were consistent with those obtained from the relative sketch data size analysis. To effectively illustrate these findings, we visualized the results using Fig.\ref{running_time_comparation_crimes} and \ref{running_time_comparation_tpch}, which showcase the impact of each strategy on query performance and efficiency.\\
From our experimental results, we observe that in most cases, the Group-by (GB) strategy emerges as the optimal choice. By employing the GB strategy, higher accuracy rates and lower relative sketch data sizes can be achieved, leading to more efficient and accurate query processing.\\
Fig.\ref{Running_time_of_reuse_over_TPCH} presents the running time overhead for different stages, including sampling, sorting, estimation, and capturing for 1ps, 2ps, 3ps, and 4ps. Since the samples and sorting results can be materialized and reused, the average overhead after these stages is acceptable. This demonstrates the feasibility of our approach in terms of computational efficiency, making it a viable option for various applications that require provenance sketches.
\subsection{Effectiveness}
			
 Firstly, We need to present the accuracy and effectiveness of our cost model based on the stratified sampling method.We create 1000 queries using the selection-aggregation template on the CRIMES, STACKOVERFLOW and TPCH. We compute the estimation relative sketch data size and the actual relative sketch data size for all queries. The number of fragments of each provenance sketch is set 1000. First, we plot the relative error which is $($estimated relative sketch data size - original relative sketch data size$)/$original relative sketch data size.
 	 They are shown as a percentage error compared with the actual relative sketch data size in Fig.\ref{relative_error_crimes} and \ref{relative_error_tpch}. The plot is based on the top 1 attribute from the provenance sketch attribute candidate based on our estimation. The result shows that for the most queries. The relative error is smaller than 1, which is acceptable.\\ 
 	 Even though our cost model will not always return the actual best provenance sketch, it can return the best estimation attribute within top 3 attribute candidate. We  plot Fig.\ref{accuracy_crimes_bar} and Fig.\ref{accuracy_tpch_bar}. The meaning of accuracy is the rate of all queries where our cost model generate the same best attribute for provenance sketch as the actual best one within top k attribute candidates. The result demonstrate that for the CRIMES our cost model will always give the best attribute for almost 100\% queries. And for TPCH, top 2 choices will give us 85\% accuracy and top 3 choices is almost 100\% accuracy. These plots give us evidence that our cost model is effective.
 	 
 	\subsection{correlation strategy}
 	correlation strategy is another pre-filtering way which can help us reduce the number of candidates of provenance sketch.
 	We first calculate the correlation matrix of the dataset attributes which is showing as heatmap in Fig. \ref{clustering_parking} Then we calculate the euclidean distance of the correlation matrix. In the next step, we use hierarchy cluster algorithms which clusters the attribute based on the euclidean distance. The average of the relative sketch data size result for each candidate in each cluster are shown in Fig.\ref{Average_relative_sketch_data_size_clustering_parking},\ref{Average_relative_sketch_data_size__clustering_crimes}. The difference of each pair in each cluster are shown in the Fig.\ref{difference_of_each_candidate_crimes},\ref{difference_of_each_candidate_parking}. For the figures, we can conclude that for some cluster. the attribute from the same cluster have the same performance, like \textbf{street\_code1} and \textbf{street\_code2} in parking and \textbf{beat} and \textbf{ward} in crimes. After we pri-filter the candidates based on the number distinct value, we can apply this correlation strategy for different queries.

 	 \subsection{Comparison}
 	 After we demonstrate our method is effective. In the next step, we plot the comparison between our cost model method and other candidate strategies which can be chosen. After getting the candidates of safe attributes to capturing provenance sketch on, different strategies can be applied to choose, including random picking from all attributes candidates, random picking from query-relatively attributes, random picking from group-by attributes, random picking from primary key attributes. random picking from aggregation attributes. The different strategies are discussed in section \ref{Strategies}.We evaluate the effective. We first plot the average relative sketch data size of 1000 queries based on the different strategies.We plot the expectation of original relative sketch data size and estimation relative sketch data size of different strategies. The results of CRIMES are shown in Fig.\ref{box_plot_crimes} and the results of TPCH are shown in Fig.\ref{box_plot_tpch}. The Fig.\ref{box_plot_crimes} and Fig.\ref{box_plot_tpch} demonstrate the actual relative sketch data size of all queries based on different strategies and the estimated relative sketch data size of all queries based on the estimated best attribute which is generated by of 5\% samples or 10\% samples. From the result, the estimated relative sketch data size results has same pattern with the original relative sketch data size results, showing the effectiveness of our cost model from other side. What's more, the pattern and the result in Fig.\ref{AVG_sketch_selectity_TPCH} and \ref{AVG_sketch_selectity_crimes} shows that generating provenance sketch candidates in the group by attributes is a good choice.
 	 
 	 \subsection{Runinng overhead}
 	 In the next step, we run the experiments focusing on the running time. We plot the Fig.\ref{running_overhead}. Even though we spend much time on the sampling, the samples can be reused if the query will run on the same tables and same provenance sketch attribute candidates where we generate the samples. The samples can be materialized. The result shows that 20 times reusing make the running overhead acceptable. 
 	 
 	 \subsection{Real World Datasets}
 	 \textbf{Chicago Crimes Dataset}
 	 \textbf{STACKOVERFLOW}
 	 \subsection{End-to-end Experiment}
 	 We want to get a rough idea of the effectiveness of our approach when we have to decide online for each incoming query which attribute is the optimal we choose to capture a provenance sketch, use a previously captured provenance sketch. experiments should contain all cost, including sorting the table, sampling, estimation time, capturing time. running original query, running query with provenance sketch. 
 	  	 \subsubsection{varying the stragtegies} 
 	  	 cb-opt,cb-opt-gb,cb-opt-rel,rand-gb, opt, 5\% sample rate
 	  	  \subsubsection{varying the vary attributes} 
 
 	  	  \subsubsection{varying query templates} 
 	   	  \subsubsection{varying the number of provenance sketch captured} 
 	   	  plot the difference of best and second ps
 	   	  materilzed sketch
 	   	  \subsubsection{test complicated query} 
 	   	  aggregation then join table and aggregates on the join results
 	\subsection{Explanation}
 	 Fig.\ref{relative_error_crimes} ,\ref{relative_error_tpch} , \ref{relative_error_parking}, \ref{relative_error_tpch_wanderjoin} and \ref{relative_error_tpch_wanderjoin3} shows a percentage error compared with the actual relative sketch data size. Relative error which is $($estimated relative sketch data size - original relative sketch data size$)/$original relative sketch data size.\\
 	 Fig.\ref{accuracy_crimes_bar} ,Fig.\ref{accuracy_tpch_bar} , \ref{accuracy_parking_bar}, \ref{accuracy_tpch_bar_wanderjoin} and \ref{accuracy_tpch_bar_wanderjoin3} shows accuracy. The meaning of accuracy is the rate of all queries where our cost model generate the same best attribute for provenance sketch as the actual best one within top k attribute candidates.\\
 	 Fig.\ref{AVG_sketch_selectity_TPCH} ,\ref{AVG_sketch_selectity_crimes} ,\ref{AVG_sketch_selectity_parking} \ref{AVG_sketch_selectity_TPCH_wanderjoin} and \ref{AVG_sketch_selectity_TPCH_wanderjoin3} shows the actual average relative sketch data size over different strategies.\\
	 Fig.\ref{box_plot_crimes}, \ref{box_plot_tpch}, \ref{box_plot_parking}, \ref{box_plot_tpch_wanderjoin} and \ref{box_plot_tpch_wanderjoin3} shows the the expectation of original relative sketch data size and estimation relative sketch data size of different strategies.\\
	 Fig.\ref{end-to-end-different-strategies} - \ref{end-to-end-different-strategies-complex-3gb} shows the end-to-end experiments results, which includes different strategies. End-to-end experiments contains capturing PS, sorting, sampling, running on the PS. ORI is the original running time. OPT is the optimal best running time. GB-Best the best attribute between the group-by attributes. RAND-GB is the average time of random picking from the group-by attributes, RAND-PK is the average time of random picking from the primary key attributes.

\section{Algorithms}

\begin{table}[H]
\begin{adjustbox}{max width=1\linewidth}
  \begin{tabular}{|l|l|}
		\hline \rowcolor{lightgrey}
		Denotation & Definition \\
		\hline
		  $O$ & current operator\\

		\hline
		  $C$ & child operator\\
		  \hline
		  $left\_C$ & left child operator\\
		  \hline
		  $right\_C$ & right child operator\\

		\hline
		  $Safe$ &  set of safe attributes\\
		  \hline
		  $T$ & input table of current operator \\
		   \hline
		  $ApproxResult$ & intermediate result\\

		\hline
		  $selection\_attr$ & set of selection attributes\\
		  \hline
		  $aggregation\_attr$ & set of selection attributes\\
		  \hline
		  $S$ & set of Selectivity of each safe atrributes\\

		\hline

  \end{tabular}
  \end{adjustbox}
  	\caption{Denotation in rules}
  \label{denotation}
    \end{table}

\begin{algorithm}[t]
  \caption{Default \textsc{selectionRules} Function}
  \begin{algorithmic}[1]
   \Procedure{selectionRules}{ $O, C, Safe$ }
	\State $selection\_attr \gets  \Call{getAttributes}{O}$
	\State $T \gets   \Call{getIntermediateResult}{C}$
	%\State $histogram \gets  \Call{getHist}{selection\_attr,table}$
	%\State $intermidateResult \gets  \Call{cost\_model\_rules}{histogram,Selection\_operator.cond}$

	\If {$\Call{noSelectionAbove}{O}$}
	\For {$attr \in Safe$}
		\State $H \gets  \Call{getHist}{selection\_attr\union attr,T}$
	  \State $ApproxResult \gets  \Call{cost\_model\_rules}{H,getSelectionCondition(O)}$
	  \State $S[attr] \gets \Call{computerSelectvity}{ApproxResult,attr}$
	 %\State $S \gets S\union S[attr]$
	\EndFor
	\Else
	\State $H \gets  \Call{getHist}{selection\_attr,T}$
	\State $ApproxResult \gets  \Call{cost\_model\_rules}{H,getSelectionCondition(O)}$
	%\State $S \gets  \Call{getProp}{C, selectivity}$
	\EndIf
   \State $\Call{storeProp}{ApproxResult} $
   \EndProcedure
   \end{algorithmic}
\end{algorithm}

\begin{algorithm}[t]
  \caption{Default \textsc{AggregationRules} Function}
  \begin{algorithmic}[1]
   \Procedure{AggregationRules}{ $O, C$ }
	\State $aggregation\_attribute,group\_by\_attribute \gets  \Call{getAttributes}{O}$
	\State $T \gets   \Call{getIntermediateResult}{C}$
	\State $attribute\_set \gets  aggregation\_attribute\union group\_by\_attribute$
	\State $H \gets  \Call{getHist}{attribute\_set,T}$
	\State $ApproxResult \gets  \Call{cost\_model\_rules}{H,getAggFunction(O)}$
	%\State $S \gets  \Call{getProp}{C, selectivity}$
	\State $\Call{storeProp}{ApproxResult}$
   \EndProcedure
   \end{algorithmic}
\end{algorithm}

\begin{algorithm}[t]
  \caption{Default \textsc{projectionRules} Function}
  \begin{algorithmic}[1]
   \Procedure{projectionRules}{ $O, C, Safe$}
   	\State $newAttrs \gets  \Call{getAttributes}{O}\union Safe$
   	\State $T \gets \Call{getIntermediateResult}{C}$

    \State $ApproxResult \gets  \projection_{newAttrs}T$

	%\State $S \gets  \Call{getProp}{C, selectivity}$
	\If {$\Call{noOperatorAbove}{this.Projection}$}
		\State \Return $\Call{minSelectivity}{S}$
	\Else
	\State $\Call{storeProp}{ApproxResult}$
	\EndIf
   \EndProcedure
   \State \Return $NULL$
   \end{algorithmic}
\end{algorithm}

\begin{algorithm}[t]
  \caption{Default \textsc{joinRules} Function}
  \begin{algorithmic}[1]
   \Procedure{projectionRules}{ $O, left\_C$}

   	\State $left\_T \gets  \Call{getIntermediateResult}{left\_C}$
   	\State $right\_T \gets  \Call{getIntermediateResult}{right\_C}$

    \State $ApproxResult \gets left\_T \join right\_T $

	%\State $S \gets \Call{getProp}{left\_C, selectivity}\union \Call{getProp}{right\_C, selectivity}$
	\State $\Call{storeProp}{ApproxResult}$

   \EndProcedure
   \end{algorithmic}
\end{algorithm}

\begin{algorithm}[t]
  \caption{Default \textsc{tableAccessRules} Function}
  \begin{algorithmic}[1]
   \Procedure{tableAccessRules}{}
	%\State $S \gets NULL$
	\State $ApproxResult \gets table$
	\State $\Call{storeProp}{ApproxResult}$

   \EndProcedure
   \end{algorithmic}
\end{algorithm}

\begin{algorithm}[t]
  \caption{Default \textsc{getHist} Function}
  \begin{algorithmic}[1]
   \Procedure{getHist}{$attributes,table$}
	\If{$\#attributes\leq2$}
	\State $H \gets \Call{getHistogram}{attributes[0],attributes[1],table}$
	\Else
	\State  $attributes \gets \Call{mergeGroupby}{attributes, correlation}$
	\For {$attr \in attributes-attributes[0]$}
	\State $H \gets H.join(\Call{get2DHistogram}{attr,attributes[0],table})$
	\EndFor
	\EndIf

   \EndProcedure
    \State \Return $H$
   \end{algorithmic}
\end{algorithm}

\begin{algorithm}[t]
  \caption{Default \textsc{checkUncertainty} Function}
  \begin{algorithmic}[1]

    \Procedure{checkUncertainty}{ $query,tables$ }
    \If{$!\Call{isSkewed}{tables}$}
      \For {$attr \in Safe$}
      \State $set \gets set \union \Call{correlation}{aggregation\_attr, attr}
$
      \EndFor
       \While{$!set.isNull$}
       \If{$!\Call{Dist\_numIsSmall}{set[0].attr,table}$}
       \State $tuples[] \gets \Call{urange}{query(compressedTable(table,pq.poll.attr))} $
       \State $filteredTables \gets \Call{filtering}{tables,tuples[]}$
       \State $break$
       \Else
       \State $set \gets set - set[0]$
       \EndIf
 	    \EndWhile
    \EndIf
    \EndProcedure
    \State \Return $filteredTables$
  \end{algorithmic}
\end{algorithm}

\begin{algorithm}[t]
  \caption{Default \textsc{isSkewed} Function}
  \begin{algorithmic}[1]
   \Procedure{isSkewed}{ $tables$ }
   	\State $getHist(attributes,table)$
   	\State $frequency = 0$
	\For {$frequency[i] \in top 10 frequent$}
	 \State $frequency \gets frequency + frequent[i]$
	\EndFor
	\If {$frequency/totalNumber \geq 10\%$}
	\State \Return $TRUE$
	 \Else
	 \State \Return $FALSE$
	 \EndIf
    \EndProcedure
         \end{algorithmic}
\end{algorithm}

\begin{algorithm}[t]
  \caption{Default \textsc{Dist\_numIsSmall} Function}
  \begin{algorithmic}[1]
   \Procedure{Dist\_numIsSmall}{ $attr,tables$ }
	\If {$distinct\_num(attr)/num(table) < 1\% $}
	\Return $TRUE$
	\Else
	\ \Return $FALSE$
	\EndIf
    \EndProcedure
         \end{algorithmic}
\end{algorithm}

\begin{algorithm}[t]
  \caption{Default \textsc{filtering} Function}
  \begin{algorithmic}[1]
   \Procedure{filtering}{ $table,tuples[]$ }
	\State $filteredTables \gets \{t^n|t^n \in table \wedge t^n\in tuples[]\} $
	\EndProcedure
         \end{algorithmic}
\end{algorithm}

\begin{algorithm}[t]
  \caption{Default \textsc{mergeGroupby} Function}
  \begin{algorithmic}[1]
   \Procedure{mergeGroupby}{ $groupby\_attrs$ }
    \State $result \gets groupby\_attrs$
	\For {$attr1 \in groupby\_attrs$}
	\For {$attr2 \in groupby\_attrs - attr$}
	\If {$\Call{correlation}{attr1,attr2} > 0.9$}
	\State $result \gets groupby\_attrs-attr2$
	\EndIf
	\EndFor
	\EndFor
	\EndProcedure
	 \State \Return $result$
    \end{algorithmic}
\end{algorithm}

%\begin{algorithm}[t]
%  \caption{Default \textsc{genNextIterChoices} Function}
%  \label{alg:gen-next-option}
%  \begin{algorithmic}[1]
%
%    \Procedure{genNextIterChoices}{ }
%      \State $p_{next} \gets p_{cur}$
%      % \State $len \gets len(p_{cur}) $
%      \For {$i \in \{ len(p_{next}), \ldots, 1\}$}
%        \State $c \gets popTail(p_{next})$
%        \State $nops \gets popTail(n_{opts})$
%        \If{$c+1 < nops$}
%          \State $c \gets c+1$
%          \State $p_{next} \gets p_{next} \cList c$
%          \State \textbf{break}
%        \EndIf
%      \EndFor
%      \State $p_{cur} \gets []$
%      \State $n_{opts} \gets []$
%    \EndProcedure
%
%  \end{algorithmic}
%\end{algorithm}

\begin{algorithm}[t]
  \caption{Default \textsc{chooseThebestAttribute} Function}
  \begin{algorithmic}[1]

    \Procedure{chooseThebestAttribute}{$tables$}
      \State $SafeAttribute \gets \Call{SafetyRule}{all\_attributes}$
      \State $histogram \gets null$
      \State $Selectivity \gets 0$
      \State $PS\_attr \gets null$
      \State $filteredTables \gets null$
       \If{$\Call{containsFilteringOp}{query}$}
      \If{$\Call{checkMonotone}{query}$}

       \For {$attr \in SafeAttribute$}
         \If{$attr \in query.selection\_attr$}
         \State $histogram \gets \Call{getHist}{1d,attr,tables}$
         \Else
         \State $histogram \gets \Call{getHist}{2d,attr,tables}$
         \EndIf
         \State $Selectivity \gets\Call{cost\_model\_rules}{histogram}$
	 	 \State $PS\_attr \gets \Call{getMinSelectivty}{Selectivity}$
       \EndFor

      \Else
         \State $filteredTables \gets \Call{checkUncertainty}{query,tables}$
          \If{$!filteredTables.isNull$}
        \State $PS\_attr \gets \Call{computeSelectivity}{filteredTables,safeAttributes}$
        \Else
        \State $PS\_attr \gets \Call{computeSelectivity}{tables,safeAttributes}$
        \EndIf

      \EndIf
      \Else
       \State $PS\_attr \gets SafeAttribute$
       \EndIf
      % \State $len \gets len(p_{cur}) $

    \EndProcedure
    \State \Return $PS\_attr$

  \end{algorithmic}
\end{algorithm}

\begin{algorithm}[t]
  \caption{Default \textsc{checkMonotone} Function}
  \begin{algorithmic}[1]

    \Procedure{checkMonotone}{$query$}
      \For {$operator \in query$}
      \If{$operator = Aggreagtion$}
      \State \Return $FALSE$
	  \EndIf
      \EndFor
    \EndProcedure
    \State \Return $TRUE$

  \end{algorithmic}
\end{algorithm}

\begin{algorithm}[t]
  \caption{Default \textsc{containsFilteringOp} Function}
  \begin{algorithmic}[1]

    \Procedure{containsFilteringOp}{$query$}
      \For {$operator \in query$}
      \If{$operator = SelctionOperator$}
      \State \Return $TRUE$
	  \EndIf
      \EndFor
    \EndProcedure
    \State \Return $FALSE$

  \end{algorithmic}
\end{algorithm}

\begin{algorithm}[t]
  \caption{Default \textsc{checkUncertainty} Function}
  \begin{algorithmic}[1]

    \Procedure{checkUncertainty}{ $query,tables$ }
    \If{$!\Call{isSkewed}{tables}$}
      \For {$attr \in SafeAttributes$}
      \State $priorityqueue\ pq.add(\Call{correlation}{query.aggregation\_attr, attr})
$
      \EndFor
       \While{$!pq.isNull$}
       \If{$!\Call{Dist\_numIsSmall}{pq.poll.attr,table}$}
       \State $tuples[] \gets \Call{urange}{query(compressedTable(table,pq.poll.attr))} $
       \State $filteredTables \gets \Call{filtering}{tables,tuples[]}$
       \State $break$
       \Else
       \State $pq.poll()$
       \EndIf
 	    \EndWhile
    \EndIf
    \EndProcedure
    \State \Return $filteredTables$
  \end{algorithmic}
\end{algorithm}

\begin{algorithm}[t]
  \caption{Default \textsc{computeSelectivity} Function}
  \begin{algorithmic}[1]

    \Procedure{computeSelectivity}{tables,safeAttributes}
   	\For {$attr \in SafeAttributes$}
   	\If {$numberGroupby>=2$}
   	\State  $groupby\_Attribute \gets \Call{mergeGroupby}{groupby\_Attribute, correlation}$
	\For {$group\_attr \in groupby\_Attribute$}
	\State $histogram \gets histogram.join(\Call{getHist}{2d,\{group\_attr,query.aggregation\_attr\},tables})$
	\EndFor
   	\Else
   	\State $histogram \gets \Call{getHist}{2d,\{group\_attr,query.aggregation\_attr\},tables}$

   	\EndIf
   	\EndFor

   	\State $Selectivity \gets\Call{cost\_model\_rules}{histogram}$
	\State $PS\_attr \gets \Call{getMinSelectivty}{Selectivity}$
    \EndProcedure
    \State \Return $PS\_attr$
  \end{algorithmic}

\end{algorithm}
